# Supplementary material for: AEGPO: Adaptive Entropy-Guided Policy Optimization for Diffusion Models
Source: arXiv:2602.06825 source file (2026-02-06)
Supplement: Supplementary file 1 [file X_suppl.tex]

\clearpage
\setcounter{page}{1}
\maketitlesupplementary

\begin{figure*}
    \centering
    \includegraphics[width=1\linewidth]{author-kit-CVPR2026-v1-latex-/appendix/图片1.png}

    \label{fig:placeholder}
\end{figure*}

\begin{figure*}
    \centering
    \includegraphics[width=1\linewidth]{author-kit-CVPR2026-v1-latex-/appendix/图片2.png}

    \label{fig:placeholder}
\end{figure*}

\begin{figure*}
    \centering
    \includegraphics[width=1\linewidth]{author-kit-CVPR2026-v1-latex-/appendix/图片3.png}

    \label{fig:placeholder}
\end{figure*}

\begin{figure*}
    \centering
    \includegraphics[width=1\linewidth]{author-kit-CVPR2026-v1-latex-/appendix/图片4.png}

    \label{fig:placeholder}
\end{figure*}

\begin{figure*}
    \centering
    \includegraphics[width=1\linewidth]{author-kit-CVPR2026-v1-latex-/appendix/图片5.png}

    \label{fig:placeholder}
\end{figure*}

\begin{figure*}
    \centering
    \includegraphics[width=1\linewidth]{author-kit-CVPR2026-v1-latex-/appendix/图片6.png}

    \label{fig:placeholder}
\end{figure*}

\begin{figure*}
    \centering
    \includegraphics[width=1\linewidth]{author-kit-CVPR2026-v1-latex-/appendix/图片7.png}

    \label{fig:placeholder}
\end{figure*}
